# Supplementary material for: Coupled cluster theory for nonadiabatic dynamics: nuclear gradients and nonadiabatic couplings in similarity constrained coupled cluster theory
Source: arXiv:2403.01007 source file (2024-05-15)
Supplement: Supplementary file 1 [file SI.pdf]

# Supporting information for "Coupled cluster theory for nonadiabatic dynamics: nuclear gradients and nonadiabatic couplings in similarity constrained coupled cluster theory"

Eirik F. Kjønstad,[1,2,3,a)] Sara Angelico,[1] and Henrik Koch[1,b)]

[1)] *Department of Chemistry, Norwegian University of Science and Technology, 7491 Trondheim, Norway*

[2)] *Department of Chemistry, Stanford University, Stanford, CA, USA*

[3)] *Stanford PULSE Institute, SLAC National Accelerator Laboratory, Menlo Park, CA, USA*

(Dated: 1 March 2024)

[a)] Electronic mail: eirik.kjonstad@ntnu.no

[b)] Electronic mail: henrik.koch@ntnu.no

## S1. ORTHOGONALITY CONDITIONS / CHOICE OF METRIC

Below, we present some results where we use other choices of projection operator than $\mathscr{E}$ and $\mathscr{K}$. One of these will be referred to as "$\mathscr{E}$ with $T = 0$" since it can be obtained from natural metric $\mathscr{E}$ by ignoring the cluster amplitudes (i.e., by setting $T = 0$). This is the simplest metric, and it is the one we used in our thymine study.[1] The effect of setting $T = 0$ is simply to enforce orthogonality between the electronic states in the singles and doubles space, that is, to require that the configuration interaction part of the coupled cluster states are orthogonal.

The other additional metric we consider will be referred to as $\mathscr{K}_5$. This metric is obtained from $\mathscr{K}$ by not only projecting on the two states, but separately projecting onto the reference, singles, and doubles contributions from the two states. The subscript "5" signifies that this constitutes a projection onto a five-dimensional space instead of the two-dimensional space obtained using $\mathscr{K}$. In general, it appears that the choice of metric is often not important and will in most cases give similar results, although in some cases the "$\mathscr{E}$ with $T = 0$" metric provides a larger correction and a poorer description (see Section S3 in particular).

## S2. MINIMUM ENERGY CONICAL INTERSECTIONS

Minimum energy conical intersections for protonated formaldimine and thymine are given in Tables S1 and S2, respectively.

| | CCSD | SCCSD | | | | XMS-CASPT2[2] | MP2/ADC(2)[2] | TDDFT[2] |
|---|---|---|---|---|---|---|---|---|
| | | ($\mathscr{S}$) | ($\mathscr{E}$) | ($\mathscr{K}$) | ($\mathscr{K}_5$) | | | |
| $S_0$ minimum | 1.271 | - | - | - | - | 1.281 | 1.275 | 1.274 |
| Planar MECI | 1.426 | 1.426 | 1.426 | 1.426 | 1.426 | 1.420 | 1.389 | 1.541 |
| Distorted MECI | 1.433 | 1.433 | 1.433 | 1.433 | 1.433 | - | - | - |

TABLE S1. C-N bond lengths (in Å) in protonated formaldimine at the $S_0$ minimum and at $S_2/S_1$ minimum energy conical intersections. The TD-DFT calculations (from Ref. 2) use the cc-pVDZ basis set. All other calculations are with the cc-pVTZ basis set.

| | $S_0$ minimum | Distorted MECI | | | | |
|---|---|---|---|---|---|---|
| | CCSD | CCSD | SCCSD | | | |
| | | | ($\mathscr{S}$) | ($\mathscr{E}$) | ($\mathscr{K}$) | ($\mathscr{K}_5$) |
| $C_4$-$O_8$ (Å) | 1.224 | 1.265* | 1.265 | 1.265 | 1.265 | 1.265 |
| $C_5$-$C_6$ (Å) | 1.357 | 1.446* | 1.446 | 1.446 | 1.446 | 1.446 |

TABLE S2. $C_4$-$O_8$ and $C_5$-$C_6$ bond lengths (in Å) for thymine at the $S_2/S_1$ minimum energy conical intersections. The $S_0$ minimum was optimized using the aug-cc-pVDZ basis. All other calculations use the cc-pVDZ basis set. The asterisk indicates that the geometry was converged only to within $10^{-3}$ a.u. in the gradient. Other geometries are converged to within $10^{-4}$ a.u.

## S3. COUPLING ELEMENTS FOR LITHIUM HYDRIDE

Coupling elements for the $2\,^1\Sigma^+/3\,^1\Sigma^+$ and $3\,^1\Sigma^+/4\,^1\Sigma^+$ states are shown in Figure S1.

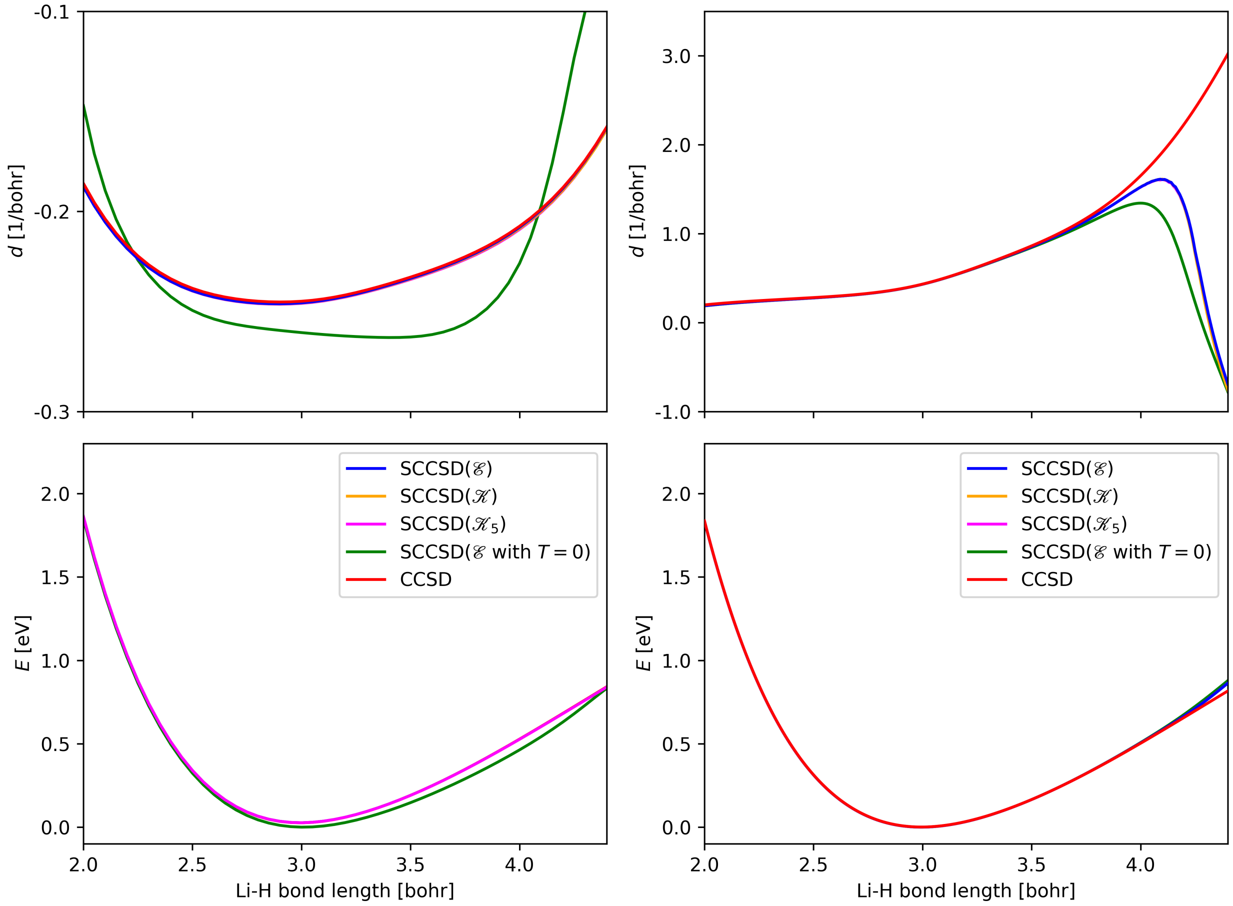


FIG. S1. Coupling elements between the $2\,^1\Sigma^+/3\,^1\Sigma^+$ (top left) and $3\,^1\Sigma^+/4\,^1\Sigma^+$ (top right) states. The magnitude of the coupling is calculated as $d = 2(d_{\mathrm{Li}} - d_{\mathrm{H}})$. Ground state energies are given in the bottom left and right panels. When evaluating the couplings, we have used the normalization described in Ref. 3 on the right coupling elements.

## S4. MULTIPLE SOLUTIONS

### A. Protonated formaldimine

In Figure S2, we present an interpolation from the Franck-Condon point to the distorted MECI of protonated formaldimine obtained by using SCCSD($\mathscr{E}$). The upper panel shows the potential energies of the two excited states involved as a function of the interpolation coordinate $x$; the bottom panel shows the value of $\zeta$ over the same range. A discontinuity in the $\zeta$ value is visible at $x \approx 0.42$, though this is not visible in the potential energy curves. In Figure S3 we present a scan of the overlap condition versus $\zeta$ at $x \approx 0.42$, revealing that the discontinuity is caused by a change of solution in the overlap condition.

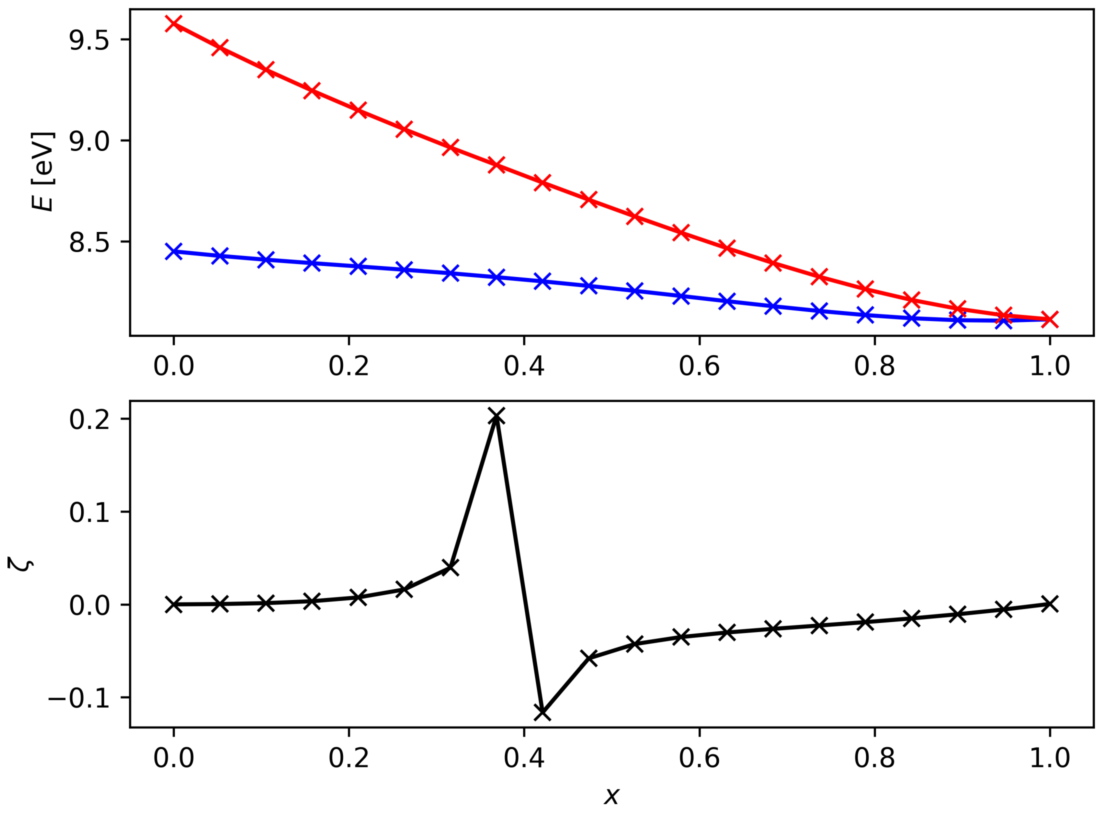


FIG. S2. Interpolation from Franck-Condon geometry ($x = 0.0$) to distorted MECI ($x = 1.0$) using SCCSD($\mathscr{E}$). At around $x \approx 0.42$, one solution of the orthogonality condition is replaced by another, as can be seen from the discontinuity in the $\zeta$ value in the lower panel.

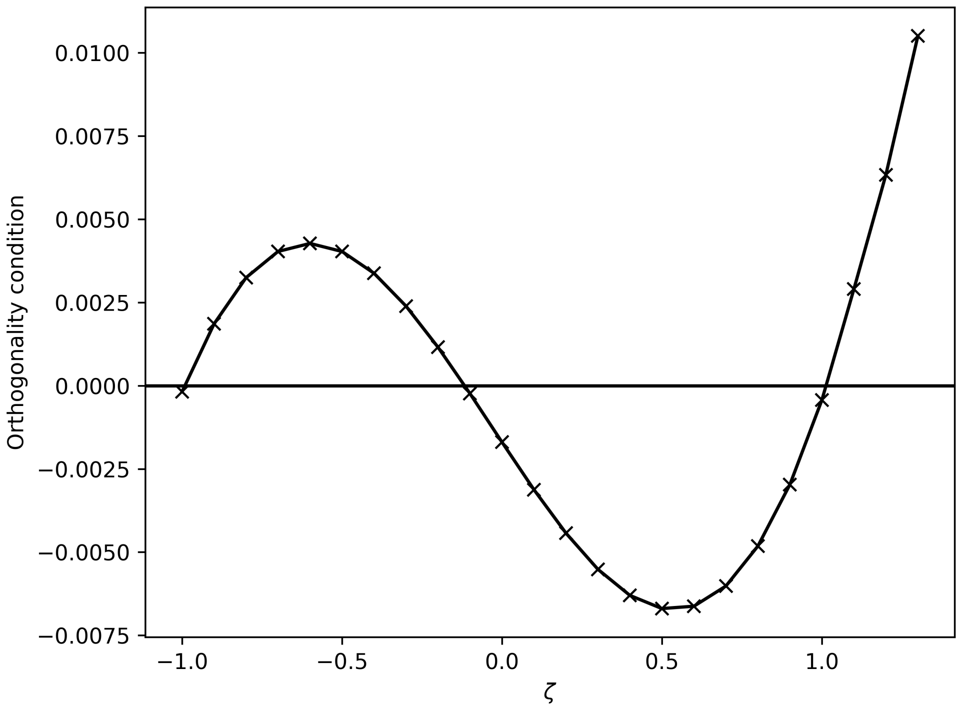


FIG. S3. The orthogonality condition as a function of $\zeta$ at the point ($x \approx 0.42$) where we see a discontinuity in the interpolation from the Franck-Condon geometry to the distorted MECI using SCCSD($\mathscr{E}$). The solution at $\zeta \approx -0.1$ is different from the solution at around $\zeta \approx 1.0$, where the latter corresponds to the solution that was obtained for the previous $x$-value ($x \approx 0.37$).

## B. Lithium hydride

Figure S4 shows the overlap condition as a function of $\zeta$ at a bond length of 4.4 bohr using SCCSD($\mathscr{E}$), where the description given by the method is already poor compared to CCSD. Here, we can see that there are two solutions, and the one giving the larger correction (at around $\zeta \approx 20$) is the one obtained in the scan shown in the main text. The other solution becomes well-behaved at bond lengths longer than 4.4 bohr.

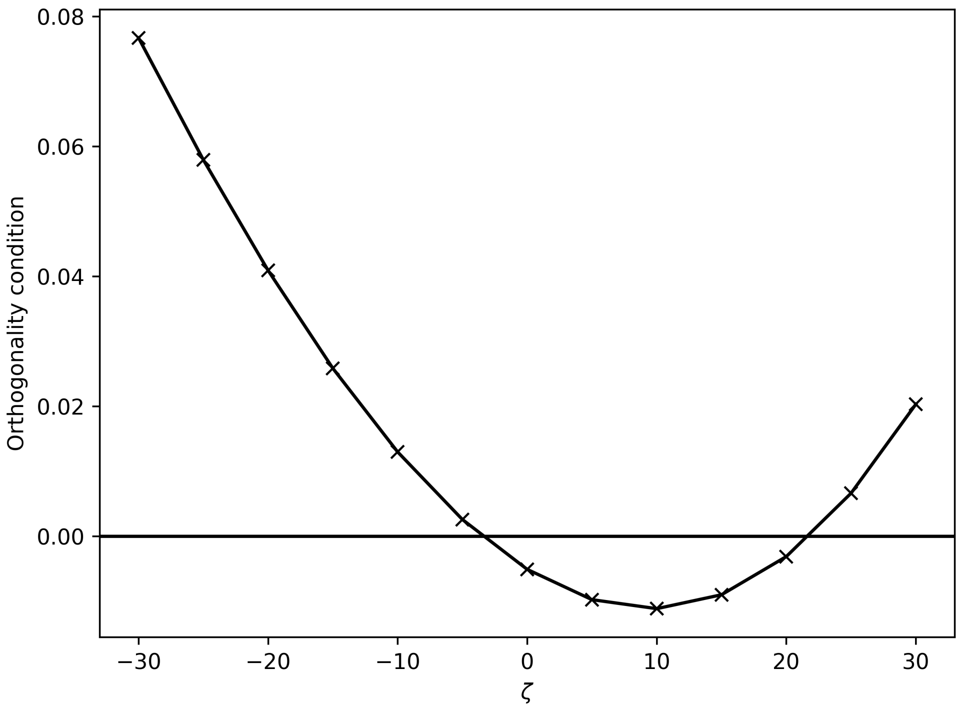


FIG. S4. The orthogonality condition as a function of $\zeta$ for LiH and SCCSD($\mathscr{E}$) at a bond distance of 4.4 bohr, where the method is already deviating significantly from CCSD. The solution at $\zeta \approx -3$ is different from the solution at around $\zeta \approx 20$, where the latter corresponds to the solution that is obtained in the scan shown in the main text. The solution at $\zeta \approx -3$ becomes well-behaved for larger bond lengths, unlike the solution at $\zeta \approx 20$.

## S5. ONE AND TWO-ELECTRON DENSITY CORRECTIONS

Here we list programmable expressions for the SCCSD corrections to the one and two-electron density matrices. We start with the one-electron matrix correction, where the only correction term is in the $ia$ block:

$$\Delta d_{ia}(\mathcal{L},\mathcal{R}) = \zeta\langle L_2|[E_{ia}, X_3]|\mathrm{HF}\rangle R_0. \tag{1}$$

To evaluate this correction, we note that

$$\begin{aligned}\Delta d_{ia}(\mathcal{L},\mathcal{R}) &= \zeta\mathscr{P}^-_{ab}\langle L_2|[E_{ia}, R_1^a R_2^b]|\mathrm{HF}\rangle R_0\\ &= \frac{\zeta}{2}R_0\mathscr{P}^-_{ab}\Delta d^{ab}_{ia}(L_2),\end{aligned} \tag{2}$$

where

$$\Delta d^{ab}_{ia}(L_2) = \Delta d^{ab}_{ia}(L_2)^a + \Delta d^{ab}_{ia}(L_2)^b + \Delta d^{ab}_{ia}(L_2)^{d_1} + \Delta d^{ab}_{ia}(L_2)^{d_2} + \Delta d^{ab}_{ia}(L_2)^f, \tag{3}$$

with

$$\Delta d^{ab}_{ia}(L_2)^a = 4L_{bjck}R^a_{bj}R^b_{aick} \tag{4}$$

$$\Delta d^{ab}_{ia}(L_2)^b = -2L_{bjcl}R^a_{bj}R^b_{cial} \tag{5}$$

$$\Delta d^{ab}_{ia}(L_2)^{d_1} = -2L_{blck}R^a_{bi}R^b_{alck} \tag{6}$$

$$\Delta d^{ab}_{ia}(L_2)^{d_2} = -2L_{ckdj}R^a_{aj}R^b_{ckdi} \tag{7}$$

$$\Delta d^{ab}_{ia}(L_2)^f = 2L_{ckdl}R^a_{ai}R^b_{ckdl}. \tag{8}$$

In the two-electron density matrix, we need to evaluate the $ijka$, $bcka$, and $iajb$ blocks. Starting with the $ijka$ block, we have

$$d_{ijka}(\mathcal{L},\mathcal{R}) = \zeta\mathscr{P}^-_{ab}\langle L_2|[e_{ijka}, R_1^a R_2^b]|\mathrm{HF}\rangle R_0 \tag{9}$$

$$= \frac{\zeta}{2}R_0\mathscr{P}^-_{ab}\Delta d_{ijka}(L_2). \tag{10}$$

Splitting into subterms, we have

$$\begin{aligned}\Delta d_{ijka}(L_2) = {}& \Delta d_{ijka}(L_2)^a + \Delta d_{ijka}(L_2)^b + \Delta d_{ijka}(L_2)^{d_1} + \Delta d_{ijka}(L_2)^{d_{2,4}}\\ &+ \Delta d_{ijka}(L_2)^{d_3} + \Delta d_{ijka}(L_2)^{e_1} + \Delta d_{ijka}(L_2)^{e_2} + \Delta d_{ijka}(L_2)^{e_3}\\ &+ \Delta d_{ijka}(L_2)^g\end{aligned} \tag{11}$$

where, first, we have for the $a$ term,

$$\Delta d_{ijka}(L_2)^a = 8\delta_{ij} Y_{ak} - 4\delta_{jk} Y_{ai} \tag{12}$$

with

$$Y_{ak} = X_{em} R^b_{akem}, \quad X_{em} = L_{emdl} R^a_{dl}. \tag{13}$$

For the $b$ term, we have

$$\Delta d_{ijka}(L_2)^b = -4\delta_{ij} Y_{ak} + 2\delta_{jk} Y_{ai} - 4Z_{jiak} + 2Z_{jkai}, \tag{14}$$

where

$$Z_{jiak} = X_{ej} \tilde{R}^b_{eiak}, \quad \tilde{R}^k_{eiak} = R^k_{eiak}(1 + \delta_{ei,ak}) \tag{15}$$

The $d_1$ term reads

$$\Delta d_{ijka}(L_2)^{d_1} = -4\delta_{ij} \tilde{Y}_{ak} + 2\delta_{jk} Z_{ai}, \tag{16}$$

where

$$Z_{ai} = X_{ad} R^a_{di}, \quad X_{ad} = L_{dnem} R^b_{anem}, \tag{17}$$

and the $d_{2,4}$ term reads

$$\Delta d_{ijka}(L_2)^{d_{2,4}} = -4\delta ij W_{ak} + 2\delta_{jk} W_{ai} - 4X_{ji} R^a_{ak} + 2X_{jk} R^a_{ai}, \tag{18}$$

where

$$W_{ak} = X_{lk} R^a_{al}, \quad X_{lk} = L_{emfl} R^b_{emfk}. \tag{19}$$

For the $d_3$ term,

$$\Delta d_{ijka}(L_2)^{d_3} = -4Y_{ijak} + 2Y_{kjai}, \tag{20}$$

where

$$Y_{ijak} = X_{ijem} R^b_{emak}, \quad X_{ijem} = L_{djem} R^a_{di}. \tag{21}$$

Considering the $e$ terms, we find for $e_1$ that

$$\Delta d_{ijka}(L_2)^{e_1} = 2Y_{ijka}, \quad Y_{ijka} = X_{ijen} R^b_{ekan}, \tag{22}$$

while for $e_2$, we have

$$\Delta d_{ijka}(L_2)^{e_2} = 2Y_{jkia}, \quad Y_{jkia} = X_{knej} R^b_{eian}, \tag{23}$$

and for $e_3$,

$$\Delta d_{ijka}(L_2)^{e_3} = 2Z_{kija}, \tag{24}$$

where

$$Z_{kija} = X_{kijl} R^a_{al}, \quad X_{kijl} = L_{elfj} R^b_{ekfi}. \tag{25}$$

The last term in the $ijka$ block, the $g$ term, reads

$$\Delta d_{ijka}(L_2)^g = N(4\delta_{ij} R^a_{ak} - 2\delta_{jk} R^a_{ai}), \tag{26}$$

where

$$N = L_{emfn} R^b_{emfn}. \tag{27}$$

Next, we move on to the $abic$ block, where we can similarly write

$$\begin{aligned}\Delta d_{abic}(L_2) = \Delta d_{abic}(L_2)^a + \Delta d_{abic}(L_2)^{b_1} + \Delta d_{abic}(L_2)^{b_2} + \Delta d_{abic}(L_2)^{c_1} \\ + \Delta d_{abic}(L_2)^{c_2} + \Delta d_{abic}(L_2)^{c_3},\end{aligned} \tag{28}$$

with, for the $a$ term,

$$\Delta d_{abic}(L_2)^a = 4Y_{ciba} - 2Y_{bica}, \quad Y_{ciba} = R^b_{cibm} X_{am}, \qquad X_{am} = L_{amck} R^a_{ck}. \tag{29}$$

For $b_1$, we have

$$\Delta d_{abic}(L_2)^{b_1} = 4Y_{ciab} - 2Y_{biac}, \quad Y_{ciab} = X_{cial} R^a_{bl}, \quad X_{cial} = R^b_{cidm} L_{dmal} \tag{30}$$

while for $b_2$, we have

$$\Delta d_{abic}(L_2)^{b_2} = 4R^a_{ci} X_{ba} - 2R^a_{bi} X_{ca}, \quad X_{ba} = R^b_{embn} L_{eman}. \tag{31}$$

For $c_1$, we get

$$\Delta d_{abic}(L_2)^{c_1} = -2Y_{cbia}, \quad Y_{cbia} = X_{iman} R^b_{cmbn}, \quad X_{iman} = R^a_{ci} L_{cman}. \tag{32}$$

For $c_2$,

$$\Delta d_{abic}(L_2)^{c_2} = -2Y_{ibac}, \quad Y_{ibac} = X_{ibal} R^a_{cl}, \quad X_{ibal} = R^b_{eibn} L_{elan} \tag{33}$$

and for $c_3$,

$$\Delta d_{abic}(L_2)^{c_3} = -2Y_{ciab}, \quad Y_{ciab} = X_{cial} R^a_{bl}, \quad X_{cial} = R^b_{cmfi} L_{fmal}. \tag{34}$$

Finally, we consider the $iajb$ block, where we first consider the term arising from the singles block $L_1$. For this contribution, we can write

$$\begin{aligned} \Delta d_{iajb}(L_1) = \mathscr{P}^{ab}_{ij}(&\Delta d_{iajb}(L_1)^a + \Delta d_{iajb}(L_1)^b \\ &+ \Delta d_{iajb}(L_1)^{c_1} + \Delta d_{iajb}(L_1)^{c_2} + \Delta d_{iajb}(L_1)^{c_3}), \end{aligned} \tag{35}$$

where, for the $a$ and $b$ terms, we have

$$\Delta d_{iajb}(L_1)^a = 2N(2R^b_{aibj} - R^b_{biaj}), \quad N = R^a_{ai} L_{ai} \tag{36}$$

and

$$\Delta d_{iajb}(L_1)^b = 8R^a_{ai} X_{bj} - 4R^a_{bi} X_{aj}, \quad X_{aj} = R^b_{ajdl} L_{dl}. \tag{37}$$

For $c_1$, we have

$$\Delta d_{iajb}(L_1)^{c_1} = -4Y_{aibj} + 2Y_{biaj}, \quad Y_{aibj} = R^b_{aibm} X_{mj}, \quad X_{mj} = L_{cm} R^a_{cj}. \tag{38}$$

For $c_2$,

$$\Delta d_{iajb}(L_1)^{c_2} = -4R^a_{ai} X_{jb} + 2R^a_{bi} X_{ja}, \quad X_{jb} = R^b_{djbm} L_{dm}, \tag{39}$$

and for $c_3$,

$$\Delta d_{iajb}(L_1)^{c_3} = -4Y_{bjai} + 2Y_{ajbi}, \quad Y_{bjai} = R^a_{bk} X_{kjai}, \quad X_{kjai} = L_{ek} R^b_{ejai}. \tag{40}$$

Next we consider the block in the $iajb$ block that stems from $L_2$. Here we have

$$\begin{aligned} \Delta d_{iajb}(L_2, R_1) = \mathscr{P}^{ab}_{ij}(&\Delta d_{iajb}(L_2, R_1)^a + \Delta d_{iajb}(L_2, R_1)^{b_1} \\ &+ \Delta d_{iajb}(L_2, R_1)^{b_{2a}} + \Delta d_{iajb}(L_2, R_1)^{b_{2b}} + \Delta d_{iajb}(L_2, R_1)^{b_{2c}} \\ &+ \Delta d_{iajb}(L_2, R_1)^{e_1} + \Delta d_{iajb}(L_2, R_1)^{e_2} + \Delta d_{iajb}(L_2, R_1)^{e_3} \\ &+ \Delta d_{iajb}(L_2, R_1)^{f_1} + \Delta d_{iajb}(L_2, R_1)^{f_2} + \Delta d_{iajb}(L_2, R_1)^{g}). \end{aligned} \tag{41}$$

For the $a$ term, we have

$$\Delta d_{iajb}(L_2, R_1)^a = 8Y_{ai}R_{bj} - 4Y_{bi}R_{aj}, \quad Y_{ai} = R^a_{ck}R^b_{dlai}L_{ckdl}. \tag{42}$$

For the $b_1$ term,

$$\Delta d_{iajb}(L_2, R_1)^{b_1} = N(4R^b_{aibj} - 2R^b_{ajbi}), \quad N = R^a_{ck}L_{ckfn}R_{fn}. \tag{43}$$

For $b_{2a}$,

$$\begin{gathered}\Delta d_{iajb}(L_2, R_1)^{b_{2a}} = -4Z_{bjai} + 2Z_{ajbi}, \quad Z_{bjai} = Y_{bd}R^b_{djai}, \\ Y_{bd} = R_{bn}X_{dn}, \quad X_{dn} = L_{dnck}R^a_{ck}.\end{gathered} \tag{44}$$

For $b_{2b}$,

$$\begin{gathered}\Delta d_{iajb}(L_2, R_1)^{b_{2b}} = -4Z_{aibj} + 2Z_{biaj}, \quad Z_{aibj} = R^b_{aibl}Y_{lj}, \\ Y_{lj} = X_{fl}R_{fj}, \quad X_{fl} = L_{flck}R^a_{ck}.\end{gathered} \tag{45}$$

For $b_{2c}$,

$$\Delta d_{iajb}(L_2, R_1)^{b_{2c}} = -4R_{ai}Y_{bj} + 2R_{bi}Y_{aj}, \quad Y_{bj} = R^b_{djbm}X_{dm}, \quad X_{dm} = L_{dmck}R^a_{ck}. \tag{46}$$

For $e_1$, we have three subterms,

$$\Delta d_{iajb}(L_2, R_1)^{e_1} = \Delta d_{iajb}(L_2, R_1)^{e_{1a}} + \Delta d_{iajb}(L_2, R_1)^{e_{1b}} + \Delta d_{iajb}(L_2, R_1)^{e_{1c}}, \tag{47}$$

where

$$\Delta d_{iajb}(L_2, R_1)^{e_{1a}} = -4Z_{aibj} + 2Z_{biaj}, \quad Z_{aibj} = R^b_{aibm}Y_{mj}, \quad Y_{mj} = X_{cm}R^a_{cj} \tag{48}$$

$$\Delta d_{iajb}(L_2, R_1)^{e_{1b}} = -4R^a_{ai}Y_{bj} + 2R^a_{bi}Y_{aj}, \quad Y_{bj} = R^b_{djbm}X_{dm} \tag{49}$$

$$\Delta d_{iajb}(L_2, R_1)^{e_{1c}} = -4Z_{bjai} + 2Z_{ajbi}, \quad Z_{bjai} = Y_{be}R^b_{ejai}, \quad Y_{be} = R^a_{bk}X_{ek}, \tag{50}$$

with

$$X_{ai} = L_{aibj}R_{bj}. \tag{51}$$

For $e_2$, we have

$$\Delta d_{iajb}(L_2, R_1)^{e_2} = \Delta d_{iajb}(L_2, R_1)^{e_{2a}} + \Delta d_{iajb}(L_2, R_1)^{e_{2b}} + \Delta d_{iajb}(L_2, R_1)^{e_{2c}}, \tag{52}$$

where

$$\Delta d_{iajb}(L_2,R_1)^{e_{2a}} = 2Z_{aijb}, \quad Z_{aijb} = Y_{aijn}R_{bn}, \quad Y_{aijn} = R^b_{alei}X_{jnel} \tag{53}$$

$$\Delta d_{iajb}(L_2,R_1)^{e_{2c}} = 2Z_{ajib}, \quad Z_{ajib} = Y_{ajin}R_{bn}, \quad Y_{ajin} = R^b_{alej}X_{inel}, \tag{54}$$

with

$$X_{inel} = R^a_{ic}L_{cnel}, \tag{55}$$

and

$$\begin{aligned}\Delta d_{iajb}(L_2,R_1)^{e_{2b}} = 2Z_{ijba}, \quad Z_{ijba} = Y_{ijkb}R^a_{ak},\\ Y_{ijkb} = X_{ijkn}R_{bn}, \quad X_{ijkn} = R^b_{djei}L_{ekdn}.\end{aligned} \tag{56}$$

Similarly, for $e_3$,

$$\Delta d_{iajb}(L_2,R_1)^{e_3} = \Delta d_{iajb}(L_2,R_1)^{e_{3a}} + \Delta d_{iajb}(L_2,R_1)^{e_{3b}} + \Delta d_{iajb}(L_2,R_1)^{e_{3c}}, \tag{57}$$

where

$$\Delta d_{iajb}(L_2,R_1)^{e_{3a}} = 2Z_{abij}, \quad Z_{abij} = R^b_{albm}Y_{lmij}, \quad Y_{lmij} = X_{ilcm}R^a_{cj} \tag{58}$$

$$\Delta d_{iajb}(L_2,R_1)^{e_{3b}} = 2Z_{aibj}, \quad Z_{aibj} = Y_{aidm}R^b_{djbm}, \quad Y_{aidm} = R^a_{ak}X_{ikdm} \tag{59}$$

$$\Delta d_{iajb}(L_2,R_1)^{e_{3c}} = 2Z_{ajib}, \quad Z_{ajib} = Y_{ajik}R^a_{bk}, \quad Y_{ajik} = R^b_{alej}X_{ilek}, \tag{60}$$

with

$$X_{ilek} = R_{ci}L_{clek}. \tag{61}$$

For $f_1$, we have

$$\Delta d_{iajb}(L_2,R_1)^{f_1} = 8Y_{ai}R^a_{bj} - 4Y_{bi}R^a_{aj}, \quad Y_{ai} = R^b_{aidl}X_{dl}, \quad X_{dl} = R_{fn}L_{dlfn}. \tag{62}$$

For $f_2$, we have

$$\begin{aligned}\Delta d_{iajb}(L_2,R_1)^{f_2} = \mathscr{P}(R_1,R^a_1)(\Delta d_{iajb}(L_2,R_1)^{f_{2a}}\\ + \Delta d_{iajb}(L_2,R_1)^{f_{2b}} + \Delta d_{iajb}(L_2,R_1)^{f_{2c}})\end{aligned} \tag{63}$$

with

$$\Delta d_{iajb}(L_2,R_1)^{f_{2a}} = -4R^a_{ai}Y_{bj} + 2R^a_{bi}Y_{aj}, \quad Y_{bj} = R_{bn}X_{jn}, \quad X_{jn} = R^b_{dleij}L_{dlen} \tag{64}$$

$$\begin{aligned}\Delta d_{iajb}(L_2,R_1)^{f_{2b}} = -4Z_{aijb} + 2Z_{bija}, \quad Z_{aijb} = Y_{aijn}R_{bn},\\ Y_{aijn} = R^b_{aidl}X_{jndl}, \quad X_{jndl} = R^a_{cj}L_{cndl}\end{aligned} \tag{65}$$

$$\Delta d_{iajb}(L_2,R_1)^{f_{2c}} = -4R_{ai}Y_{bj} + 2R_{bi}Y_{aj}, \quad Y_{bj} = X_{bc}R^a_{cj}, \quad X_{bc} = R^b_{bmdl}L_{cmdl}. \tag{66}$$

Finally, for the $g$ term, we have

$$\Delta d_{iajb}(L_2, R_1)^g = N(4R^a_{ai}R_{bj} - 2R^a_{bi}R_{aj}), \quad N = R^b_{dlem}L_{dlem}. \tag{67}$$

Although the terms above give the SCCSD corrections to densities relative to CCSD, there are also some additional Hartree-Fock level density terms that enter into the nuclear derivatives. These terms arise because of the reference term in the overlap ($R^k_0$), which produces a reference contributions to the effective SCCSD density matrices. In particular, the Lagrangians have the term

$$\bar{L}^k_0 \langle \mathrm{HF} \,|\, \bar{H} \,|\, \mathcal{R}_k \rangle \tag{68}$$

which implies density contributions of the form

$$\langle \mathrm{HF} \,|\, E_{pq} \,|\, \mathrm{HF} \rangle \tag{69}$$

$$\langle \mathrm{HF} \,|\, e_{pqrs} \,|\, \theta \rangle, \quad |\theta\rangle = \sum_{\mu} \theta_\mu |\mu\rangle. \tag{70}$$

These Hartree-Fock density contributions are well-known and we refer to the literature for programmable expressions.[4]

## S6. RESPONSE VECTORS FOR EXCITED STATE STATIONARITY

Let us start with

$$\rho_\mu^m = \langle\bar{\zeta}|Y_\mu^m|\mathrm{HF}\rangle. \tag{71}$$

We have

$$\begin{aligned}\rho_{ai}^m &= \zeta\langle\bar{\zeta}|[\hat{H}, E_{ai}R_2^n]|\mathrm{HF}\rangle \\ &= \frac{1}{2}\zeta\bar{R}_{bjck}^n\langle\bar{\zeta}|[H, E_{ai}E_{bj}E_{ck}|\mathrm{HF}\rangle \\ &= \frac{1}{2}\zeta\bar{R}_{bjck}^n\omega_{ijk}^{abc},\end{aligned} \tag{72}$$

where

$$\omega_{ijk}^{abc} = \sum_{\alpha=1}^{7} {}^{\alpha}\omega_{ijk}^{abc} \tag{73}$$

with

$$\begin{aligned}
{}^1\omega_{ijk}^{abc} &= 2\bar{\zeta}_{aibj}F_{kc} \\
{}^2\omega_{ijk}^{abc} &= 2\bar{\zeta}_{ai}L_{jbkc} \\
&\quad - P_{jk}^{bc}(F_{jc}\bar{\zeta}_{aibk} + L_{jlkc}\bar{\zeta}_{aibl} - L_{dbkc}\bar{\zeta}_{aidj}) \\
{}^3\omega_{ijk}^{abc} &= 2\bar{\zeta}_{aick}F_{jb} \\
{}^4\omega_{ijk}^{abc} &= 2\bar{\zeta}_{bj}L_{iakc} \\
&\quad - P_{ik}^{ac}(F_{ic}\bar{\zeta}_{bjak} + L_{ilkc}\bar{\zeta}_{bjal} - L_{dakc}\bar{\zeta}_{bjdi}) \\
{}^5\omega_{ijk}^{abc} &= P_{ijk}^{abc}(-L_{jbic}\bar{\zeta}_{ak} + g_{iljc}\bar{\zeta}_{albk} - g_{ibdc}\bar{\zeta}_{djak}) \\
{}^6\omega_{ijk}^{abc} &= 2\bar{\zeta}_{ck}L_{iajb} \\
&\quad - P_{ij}^{ab}(F_{ib}\bar{\zeta}_{ckaj} + L_{iljb}\bar{\zeta}_{ckal} - L_{dajb}\bar{\zeta}_{ckdi}) \\
{}^7\omega_{ijk}^{abc} &= 2\bar{\zeta}_{bjck}F_{ia}.
\end{aligned} \tag{74}$$

Similarly,

$$\begin{aligned}\rho_{aibj}^m &= -\zeta\langle\bar{\zeta}|[\hat{H}, E_{ai}E_{bj}R_1^n]|\mathrm{HF}\rangle \\ &= -\zeta R_{ck}^n\omega_{ijk}^{abc},\end{aligned} \tag{75}$$

so that we may reuse the formula for $\omega_{ijk}^{abc}$. Note that, in order to avoid $N^7$ scaling, we do not implement $\omega_{ijk}^{abc}$ but rather its partial contractions with $R_{ck}^n$ and $R_{bjck}^n$.

Next we consider

$$\sigma_\mu^m = \langle \Lambda | [Y_\mu^m, R] | \mathrm{HF} \rangle. \tag{76}$$

Here we also define a useful tensor:

$$\begin{aligned} \sigma_{ai}^m &= \zeta \langle \Lambda | [[\hat{H}, E_{ai} R_2^n], R_1] | \mathrm{HF} \rangle \\ &= \frac{\zeta}{2} \bar{R}_{bjck}^n R_{dl} \langle \Lambda | [[\hat{H}, E_{ai} E_{bj} E_{ck}], E_{dl}] | \mathrm{HF} \rangle \\ &= \frac{\zeta}{2} \bar{R}_{bjck}^n R_{dl} \gamma_{ijkl}^{abcd}. \end{aligned} \tag{77}$$

This tensor also has 7 terms,

$$\gamma_{ijkl}^{abcd} = \sum_{\alpha=1}^{7} {}^{\alpha}\gamma_{ijkl}^{abcd}, \tag{78}$$

with

$${}^{1}\gamma_{ijkl}^{abcd} = 2\Lambda_{aibj} L_{kcld} \tag{79}$$

$${}^{2}\gamma_{ijkl}^{abcd} = -P_{jkl}^{bcd} L_{kcjd} \Lambda_{aibl} \tag{80}$$

$${}^{3}\gamma_{ijkl}^{abcd} = 2\Lambda_{aick} L_{jbld} \tag{81}$$

$${}^{4}\gamma_{ijkl}^{abcd} = -P_{ikl}^{acd} L_{kcid} \Lambda_{bjal} \tag{82}$$

$${}^{5}\gamma_{ijkl}^{abcd} = P_{ijk}^{abc} (g_{kbid} \Lambda_{cjal} + g_{lbic} \Lambda_{djak}) \tag{83}$$

$${}^{6}\gamma_{ijkl}^{abcd} = -P_{jil}^{bad} L_{iajd} \Lambda_{ckbl} \tag{84}$$

$${}^{7}\gamma_{ijkl}^{abcd} = 2\Lambda_{bjck} L_{iald}. \tag{85}$$

Again, we obtain expressions by using that

$$\begin{aligned} \sigma_{aibj}^m &= -\zeta \langle \Lambda | [[H, E_{ai} E_{bj} R_1^n], R_1] | \mathrm{HF} \rangle \\ &= -\zeta R_{ck}^n R_{dl} \gamma_{ijkl}^{abcd}. \end{aligned} \tag{86}$$

It is useful to explicitly denote the dependence of these vectors, i.e. by writing

$$\rho_\mu^m = \rho_\mu^m(\bar{\zeta}) \tag{87}$$

$$\sigma_\mu^m = \sigma_\mu^m(\Lambda, R). \tag{88}$$

In particular, this allows to see that

$$R_\mu^m \rho_\mu^m(\bar{\zeta}) = \zeta \langle \bar{\zeta} | [\hat{H}, X_3] | \mathrm{HF} \rangle \tag{89}$$

$$R_\mu^m \sigma_\mu^m(\Lambda, R) = \zeta \langle \Lambda | [[\hat{H}, X_3], R] | \mathrm{HF} \rangle \tag{90}$$

and hence we can calculate the $\zeta$-derivative terms (in $\partial\mathscr{L}_n/\partial\zeta$) by reusing the code from the state derivatives and then evaluate the response by evaluating the dot products in Eqs. (89) and (90), appropriately premultiplying by $\zeta^{-1}$.

## S7. RESPONSE CONTRIBUTIONS FROM THE ORTHOGONALITY

When differentiating the orthogonality condition, we can in most cases reuse expressions implemented in the original SCCSD paper.[5] The single exception is the $t_\mu$ derivative, which gives rise to terms of the form

$$\langle \mathcal{L} | \tau_\mu \exp(T) | \mathcal{R} \rangle = L_\mu R_0 + \sum_\nu \langle \mathcal{L} | \tau_\mu | \nu \rangle \langle \nu | \exp(T) | \mathcal{R} \rangle \tag{91}$$

$$= L_\mu R_0 + \langle L | \tau_\mu | q \rangle R_0 + \langle L | \tau_\mu | QR \rangle \tag{92}$$

$$= L_\mu R_0 + J_\mu(L, q) R_0 + J_\mu(L, QR), \tag{93}$$

where

$$|q\rangle = \sum_\mu q_\mu |\mu\rangle, \quad q_\mu = \langle \mu | \exp(T) | \mathrm{HF} \rangle \tag{94}$$

and

$$|QR\rangle = \sum_\mu (\boldsymbol{QR})_\mu |\mu\rangle, \quad Q_{\mu\nu} = \langle \mu | \exp(T) | \nu \rangle. \tag{95}$$

Programmable expressions for $\boldsymbol{J}$ are given in Ref. 3 and for $\boldsymbol{q}$ and $\boldsymbol{Q}$, as well as the terms needed to evaluate the relevant vectors $\langle \mathcal{L}|$ and $|\mathcal{R}\rangle$, we refer to Ref. 5.

## REFERENCES

[1]E. F. Kjønstad, O. J. Fajen, A. C. Paul, S. Angelico, D. Mayer, M. Gühr, T. J. A. Wolf, T. J. Martínez, and H. Koch, "Unexpected hydrogen dissociation in thymine: predictions from a novel coupled cluster theory," To be submitted. (2024).

[2]J. T. Taylor, D. J. Tozer, and B. F. E. Curchod, "On the description of conical intersections between excited electronic states with LR-TDDFT and ADC(2)," J. Chem. Phys. **159**, 214115 (2023).

[3]E. F. Kjønstad and H. Koch, "Communication: Non-adiabatic derivative coupling elements for the coupled cluster singles and doubles model," J. Chem. Phys. **158**, 161106 (2023).

[4]T. Helgaker, P. Jorgensen, and J. Olsen, *Molecular electronic-structure theory* (John Wiley & Sons, 2013).

[5]E. F. Kjønstad and H. Koch, "An orbital invariant similarity constrained coupled cluster model," J. Chem. Theory Comput. **15**, 5386–5397 (2019).
